# Supplementary material for: To Patch, or not To Patch? That is the Question: A Case Study of System Administrators' Online Collaborative Behaviour
Source: arXiv:2307.03609 source file (2023-07-07)
Supplement: Supplementary file 1 [file Appendix.tex]

\begin{table}[t]
\begin{center}
\resizebox{1\columnwidth}{!}{
\large
\begin{tabular}{|l|l|l|l|l|}
\hline
\textbf{Patch} & \textbf{CVE} & \textbf{Severity} & \textbf{Impact} & \textbf{Product} \\ \hline
KB4034664 and KB4024679 & CVE-2017-8624 & Important & Elevation of Privilege & Windows 7 SP 1 and Windows Server 2008 R2 SP 1 \\ \hline
KB4034664 and KB4024679 & CVE-2017-8633 & Important & Elevation of Privilege & Windows 7 SP 1 and Windows Server 2008 R2 SP 1 \\ \hline
KB4034664 and KB4024679 & CVE-2017-0174 & Important & Denial of Service & Windows 7 SP 1 and Windows Server 2008 R2 SP 1 \\ \hline
KB4034664 and KB4024679 & CVE-2017-0293 & Critical & Remote Code Execution & Windows 7 SP 1 and Windows Server 2008 R2 SP 1 \\ \hline
KB4034664 and KB4024679 & CVE-2017-8593 & Important & Elevation of Privilege & Windows 7 SP 1 and Windows Server 2008 R2 SP 1 \\ \hline
KB4034664 and KB4024679 & CVE-2017-8620 & Critical & Remote Code Execution & Windows 7 SP 1 and Windows Server 2008 R2 SP 1 \\ \hline
KB4034664 and KB4024679 & CVE-2017-8666 & Important & Information Disclosure & Windows 7 SP 1 and Windows Server 2008 R2 SP 1 \\ \hline
KB4034664 and KB4024679 & CVE-2017-8668 & Important & Information Disclosure & Windows 7 SP 1 and Windows Server 2008 R2 SP 1 \\ \hline
KB4034664 and KB4024679 & CVE-2017-8691 & Important & Remote Code Execution & Windows 7 SP 1 and Windows Server 2008 R2 SP 1 \\ \hline
KB4034664 & CVE-2017-8635 & Moderate & Remote Code Execution & Internet Explorer 11 \\ \hline
KB4034664 & CVE-2017-8636 & Moderate & Remote Code Execution & Internet Explorer 11 \\ \hline
KB4034664 & CVE-2017-8641 & Moderate & Remote Code Execution & Internet Explorer 11 \\ \hline
KB4034664 & CVE-2017-8653 & Moderate & Remote Code Execution & Internet Explorer 11 \\ \hline
KB4034664 & CVE-2017-8669 & Moderate & Remote Code Execution & Internet Explorer 11 \\ \hline
\end{tabular}%
}
\caption{Vulnerabilities addressed by KB's 4034679 and 4034664.}
\label{tab:tabelVuln}
\end{center}
\end{table}
